# Supplementary material for: Large Language Models are In-Context Molecule Learners
Source: arXiv:2403.04197 source file (2025-04-07)
Supplement: Supplementary file 1 [file appendix.tex]

\newpage
\section{Appendix}

\subsection{Hyper Parameters}
Table \ref{tab:hyper} illustrates all the hyperparameters and their corresponding value ranges. The first part is about the general training settings and ICMA settings. Notably, if not specifically stated, the default cutoff length is set to 1024, and the n\_shot (i.e., number of context examples) is set to 2. Next, Lora and acceleration settings are listed. Lastly, we also provide the hyperparameters for controlling the generation.
\begin{table}[htb]
    \centering
    \begin{tabular}{c|c}
    \toprule
    Item & Value \\
    \midrule
    batch size & 32  \\
    epochs & 10 \\
    warm-up steps & 1000 \\
    cutoff length & 512, 1024, 1536, 2048 \\
    n\_shot & 1,2,3,4 \\
    learning rate & 2e-4 \\
    \midrule
    lora\_r & 32\\
    lora\_alpha & 64 \\
    lora\_dropout & 0.1 \\
    int8 & True \\
    fp16 & True \\
    \midrule
    temperature & 0.7 \\
    top\_p & 0.85 \\
    top\_k & 40 \\
    num\_beams & 1 \\
    max\_new\_tokens & 256 \\
    \bottomrule
    \end{tabular}
    \caption{Hyper-Parameters}
    \label{tab:hyper}
\end{table}
\subsection{Context Templates}
Next, we introduce the context templates adopted to form the input of LLMs. Generally, the context templates are much simpler than those in MolReGPT because LLMs are fine-tuned in ICMA, which makes it easier for output-format control. In this case, the format control prompts could be omitted. At the same time, we still add proper prompts before generation to motivate LLMs to learn from the context examples, especially identifying the similarities and differences within these context examples.

\noindent \textbf{Cap2Mol ICMA Prompt}
\hrule
\noindent Generate a caption for the molecule: 
\noindent \{PlaceHolder\}

\noindent Caption: \{PlaceHolder\}

\noindent ...

\noindent Based on the above examples, analyse the similarities and differences between the examples and finally generate a caption for the molecule: \{PlaceHolder\}. 

\noindent Caption: \{For Generation\}
\hrule
\noindent \textbf{Mol2Cap ICMA Prompt}
\hrule
\noindent Generate a molecule for the caption: 
\noindent \{PlaceHolder\}

\noindent Molecule:\{PlaceHolder\}

\noindent ...

\noindent Based on the above examples, analyse the similarities and differences between the examples and finally generate a molecule for the caption: \{PlaceHolder\}. 

\noindent Molecule: \{For Generation\}
\hrule

\subsection{Further Discussion}
In this section, we conduct some further experiments to provide extra insights and support our method. First, we test and compare the performances of different backbone LLMs with and without ICMA. Then, we compare ICMA with some other baseline models.

\subsubsection{Results with More Backbone LLMs}
To highlight the model agnosticism of ICMA, we have expanded our experiments on two more backbone LLMs, Galactica-1.3B and Llama-2-7b-chat-hf. The results are shown in Tables \ref{tab:m2c_more} and \ref{tab:c2m_more}. It is evident that ICMA enhances the performance of both models, which further proves the versatility of ICMA.
\begin{table}[htbp]
    \centering

    \resizebox{1.0\columnwidth}{!}{
    \begin{tabular}{c|c|c|c|c|c|c}
    \toprule
    Backbone & BLEU-2$\uparrow$ & BLEU-4$\uparrow$ & ROUGE-1$\uparrow$ & ROUGE-2$\uparrow$ & ROUGE-L$\uparrow$ & METEOR$\uparrow$ \\
    \midrule
    Galactica-1.3B & 0.589 &	0.507 &	0.638 &	0.484 &	0.574 &	0.597 \\ 
    ICMA(Galactica-1.3B) & 0.602 &	0.534 &	0.668 &	0.530 &	0.607 &	0.649 \\ 
    Llama2-7B & 0.515 &	0.423 &	0.583 &	0.412 &	0.518 &	0.528\\
    ICMA(Llama2-7B) & 0.629 &	0.553 &	0.663 &	0.518 &	0.601 &	0.635\\
    \bottomrule
    \end{tabular}
    }
    \vskip -0.1in
    \caption{Performance comparison of more backbone LLMs for Mol2Cap task on ChEBI-20 dataset. Here, we select Galactica-1.3B and Llama-2-7b-chat-hf for demonstration.}
    \vskip -0.1in
    \label{tab:m2c_more}
\end{table}

\begin{table}[htbp]
    \centering
    \resizebox{1.0\columnwidth}{!}{
    \begin{tabular}{c|c|c|c|c|c|c|c}
    \toprule
    Backbone & BLEU$\uparrow$ & EM$\uparrow$ & Levenshtein$\downarrow$ & MACCS FTS$\uparrow$ & RDK FTS$\uparrow$ & Morgan FTS$\uparrow$ & Validity$\uparrow$ \\
    \midrule
    Galactica-1.3B & 0.812 & 0.292 &	22.47 &	0.882 &	0.777 &	0.709 &	0.950 \\
    ICMA(Galactica-1.3B) &  0.839 &	0.396 &	21.61 &	0.910 &	0.829 &	0.770 &	0.946 \\
    Llama2-7B & 0.663 &	0.130 &	37.24 &	0.801 &	0.649 &	0.572 &	0.861\\
    ICMA(Llama2-7B) & 0.783 &	0.319 &	27.74 &	0.888 &	0.792 &	0.727 &	0.923 \\
    \bottomrule
    \end{tabular}
    }
    \vskip -0.1in
    \caption{Performance comparison of more backbone LLMs for Cap2Mol task on ChEBI-20 dataset. Here, we select Galactica-1.3B and Llama-2-7b-chat-hf for demonstration.}
    \label{tab:c2m_more}
    \vskip -0.2in
\end{table}

\subsubsection{Comparison with Other Baseline Models}
In our pursuit to comprehensively evaluate the efficacy of ICMA, we have extended our comparative analysis to include additional baseline models. Specifically, we first compare ICMA(Mistral-7B) with BioT5 ~\cite{pei2023biot5}, ~\cite{liu2023molxpt}, and MolCA ~\cite{liu2023molca} in the \textbf{Mol2Cap} task. The results, as detailed in Table \ref{tab:m2c_morebase}, indicate that ICMA outperforms all the baseline models in terms of BLEU-2, BLEU-4, and METEOR scores, while also achieving the second-highest ROUGE scores, which further prove that ICMA could empower Mistral-7B to achieve SOTA or comparable performance. 

Notably, compared to MolCA, a multi-modal method that leverages 2D molecular graphs to augment LLMs for the Mol2Cap task, our ICMA is capable of refining the alignment between molecular and textual representations not only for Mol2Cap task but also for Cap2Mol task, which is more important to the field of molecule discovery.

Furthermore, for the \textbf{Cap2Mol} task, we have included BioT5 ~\cite{pei2023biot5} and MolXPT ~\cite{liu2023molxpt} in our comparative analysis. As presented in Table \ref{tab:c2m_morebase}, ICMA achieves the highest scores in exact match and molecule fingerprints metrics, indicative of superior quality in molecule generation.  However, it is also important to note that since the Mistral-7B model was not pre-trained on a large-scale chemical corpus, the validity of the generation is slightly below the two baseline models due to a deficiency in molecular knowledge.

\begin{table*}[htbp]
    \centering

    \resizebox{1.5\columnwidth}{!}{
    \begin{tabular}{c|c|c|c|c|c|c}
    \toprule
    Backbone & BLEU-2$\uparrow$ & BLEU-4$\uparrow$ & ROUGE-1$\uparrow$ & ROUGE-2$\uparrow$ & ROUGE-L$\uparrow$ & METEOR$\uparrow$ \\
    \midrule
    BioT5 ~\cite{pei2023biot5} & \underline{0.635} &	\underline{0.556} &	\textbf{0.692} &	\textbf{0.559} &	\textbf{0.633} &	\underline{0.656} \\ 
    MolXPT ~\cite{liu2023molxpt} & 0.594 &	0.505 &	0.660 &	0.511 &	0.597 &	0.626 \\ 
    MolCA ~\cite{liu2023molca} & 0.620 &	0.531 &	0.681 &	0.537 &	0.618 &	0.651\\
    ICMA(Mistral-7B) & \textbf{0.651} &	\textbf{0.581} & \underline{0.686} & \underline{0.550} &	\underline{0.625} 	& \textbf{0.661} \\
    \bottomrule
    \end{tabular}
    }
    \caption{Performance comparison with more baseline models for Mol2Cap task on ChEBI-20 dataset. Here, we select BioT5 ~\cite{pei2023biot5}, MolXPT ~\cite{liu2023molxpt}, and MolCA ~\cite{liu2023molca} for comparison.}
    \label{tab:m2c_morebase}
\end{table*}

\begin{table*}[htbp]
    \centering
    \resizebox{1.5\columnwidth}{!}{
    \begin{tabular}{c|c|c|c|c|c|c|c}
    \toprule
    Backbone & BLEU$\uparrow$ & EM$\uparrow$ & Levenshtein$\downarrow$ & MACCS FTS$\uparrow$ & RDK FTS$\uparrow$ & Morgan FTS$\uparrow$ & Validity$\uparrow$ \\
    \midrule
    BioT5 ~\cite{pei2023biot5}& \textbf{0.867} & \underline{0.413} &	\textbf{15.10} &	\underline{0.886} &	\underline{0.801} &	\underline{0.734} & \textbf{1.000} \\
    MolXPT ~\cite{liu2023molxpt}& - & 0.215 &	22.47 &	0.859 &	0.757 &	0.667 &	\underline{0.983} \\
    ICMA(Mistral-7B) & \underline{0.855} & 	\textbf{0.460} &	\underline{18.73} &	\textbf{0.916} &	\textbf{0.837} &	\textbf{0.789} & 0.958  \\
    \bottomrule
    \end{tabular}
    }
    \caption{Performance comparison of more baseline models for Cap2Mol task on ChEBI-20 dataset. Here, we include the results from BioT5 ~\cite{pei2023biot5} and MolXPT ~\cite{liu2023molxpt} for comparison.}
    \label{tab:c2m_morebase}
\end{table*}

\subsection{Case Study}
Here, we demonstrate the performance of different methods by introducing detailed examples in both the Cap2Mol and Mol2Cap sub-tasks. 

\noindent\textbf{Cap2Mol} Figure \ref{fig:case_c2m} showcases a series of molecule examples produced by various baseline methods and our proposed approach, ICMA. In the first example, both MolT5 and MolReGPT exhibited errors in the positions of functional groups, while ICMA precisely replicated the correct structure. Meanwhile, in the third example, MolT5 and MolReGPT made a mistake in the type of functional groups, generating an $[NH_2]^+$ instead of the $[NH]$. What's more, across the remaining examples, ICMA could even better match the number of carbon atoms in the SMILES representations of molecules, which consistently demonstrated superior proficiency in capturing the intricate alignment between natural language descriptions and molecule structures, thereby proving the efficacy of our proposed method.

\noindent\textbf{Mol2Cap} Figure \ref{fig:case_m2c} presents a set of caption examples produced by two baseline methods and our ICMA. In the first example, MolT5 incorrectly equated \emph{D-tartrate(2-)} with \emph{L-tartrate(2-)} and \emph{L-tartrate(1-)} with \emph{D-tartrate(1-)}, while MolReGPT introduced an excessive amount of irrelevant information. In contrast, ICMA could accurately empower backbone models to generate precise answers. Meanwhile, in the second example, ICMA accurately recognized that the molecule in question \emph{"has a role as an antibacterial drug"}, whereas MolReGPT failed. Moreover, in the fourth example, ICMA meticulously captured all the essential details in describing the molecule structures without a single mistake, demonstrating that contextual examples can significantly enhance the understanding of molecule structures, especially the types and positions of functional groups.

To summarize, ICMA could fine-grain the detailed alignment between molecule captions and molecule SMILES representations via learning from context examples. ICMA could match the types and positions of functional groups, the number of carbon atoms, as well as the overall structures more accurately, showing that LLMs are inherently in-context molecule learners.

\begin{figure*}[htb]
    \centering
    
    \includegraphics[width=\textwidth]{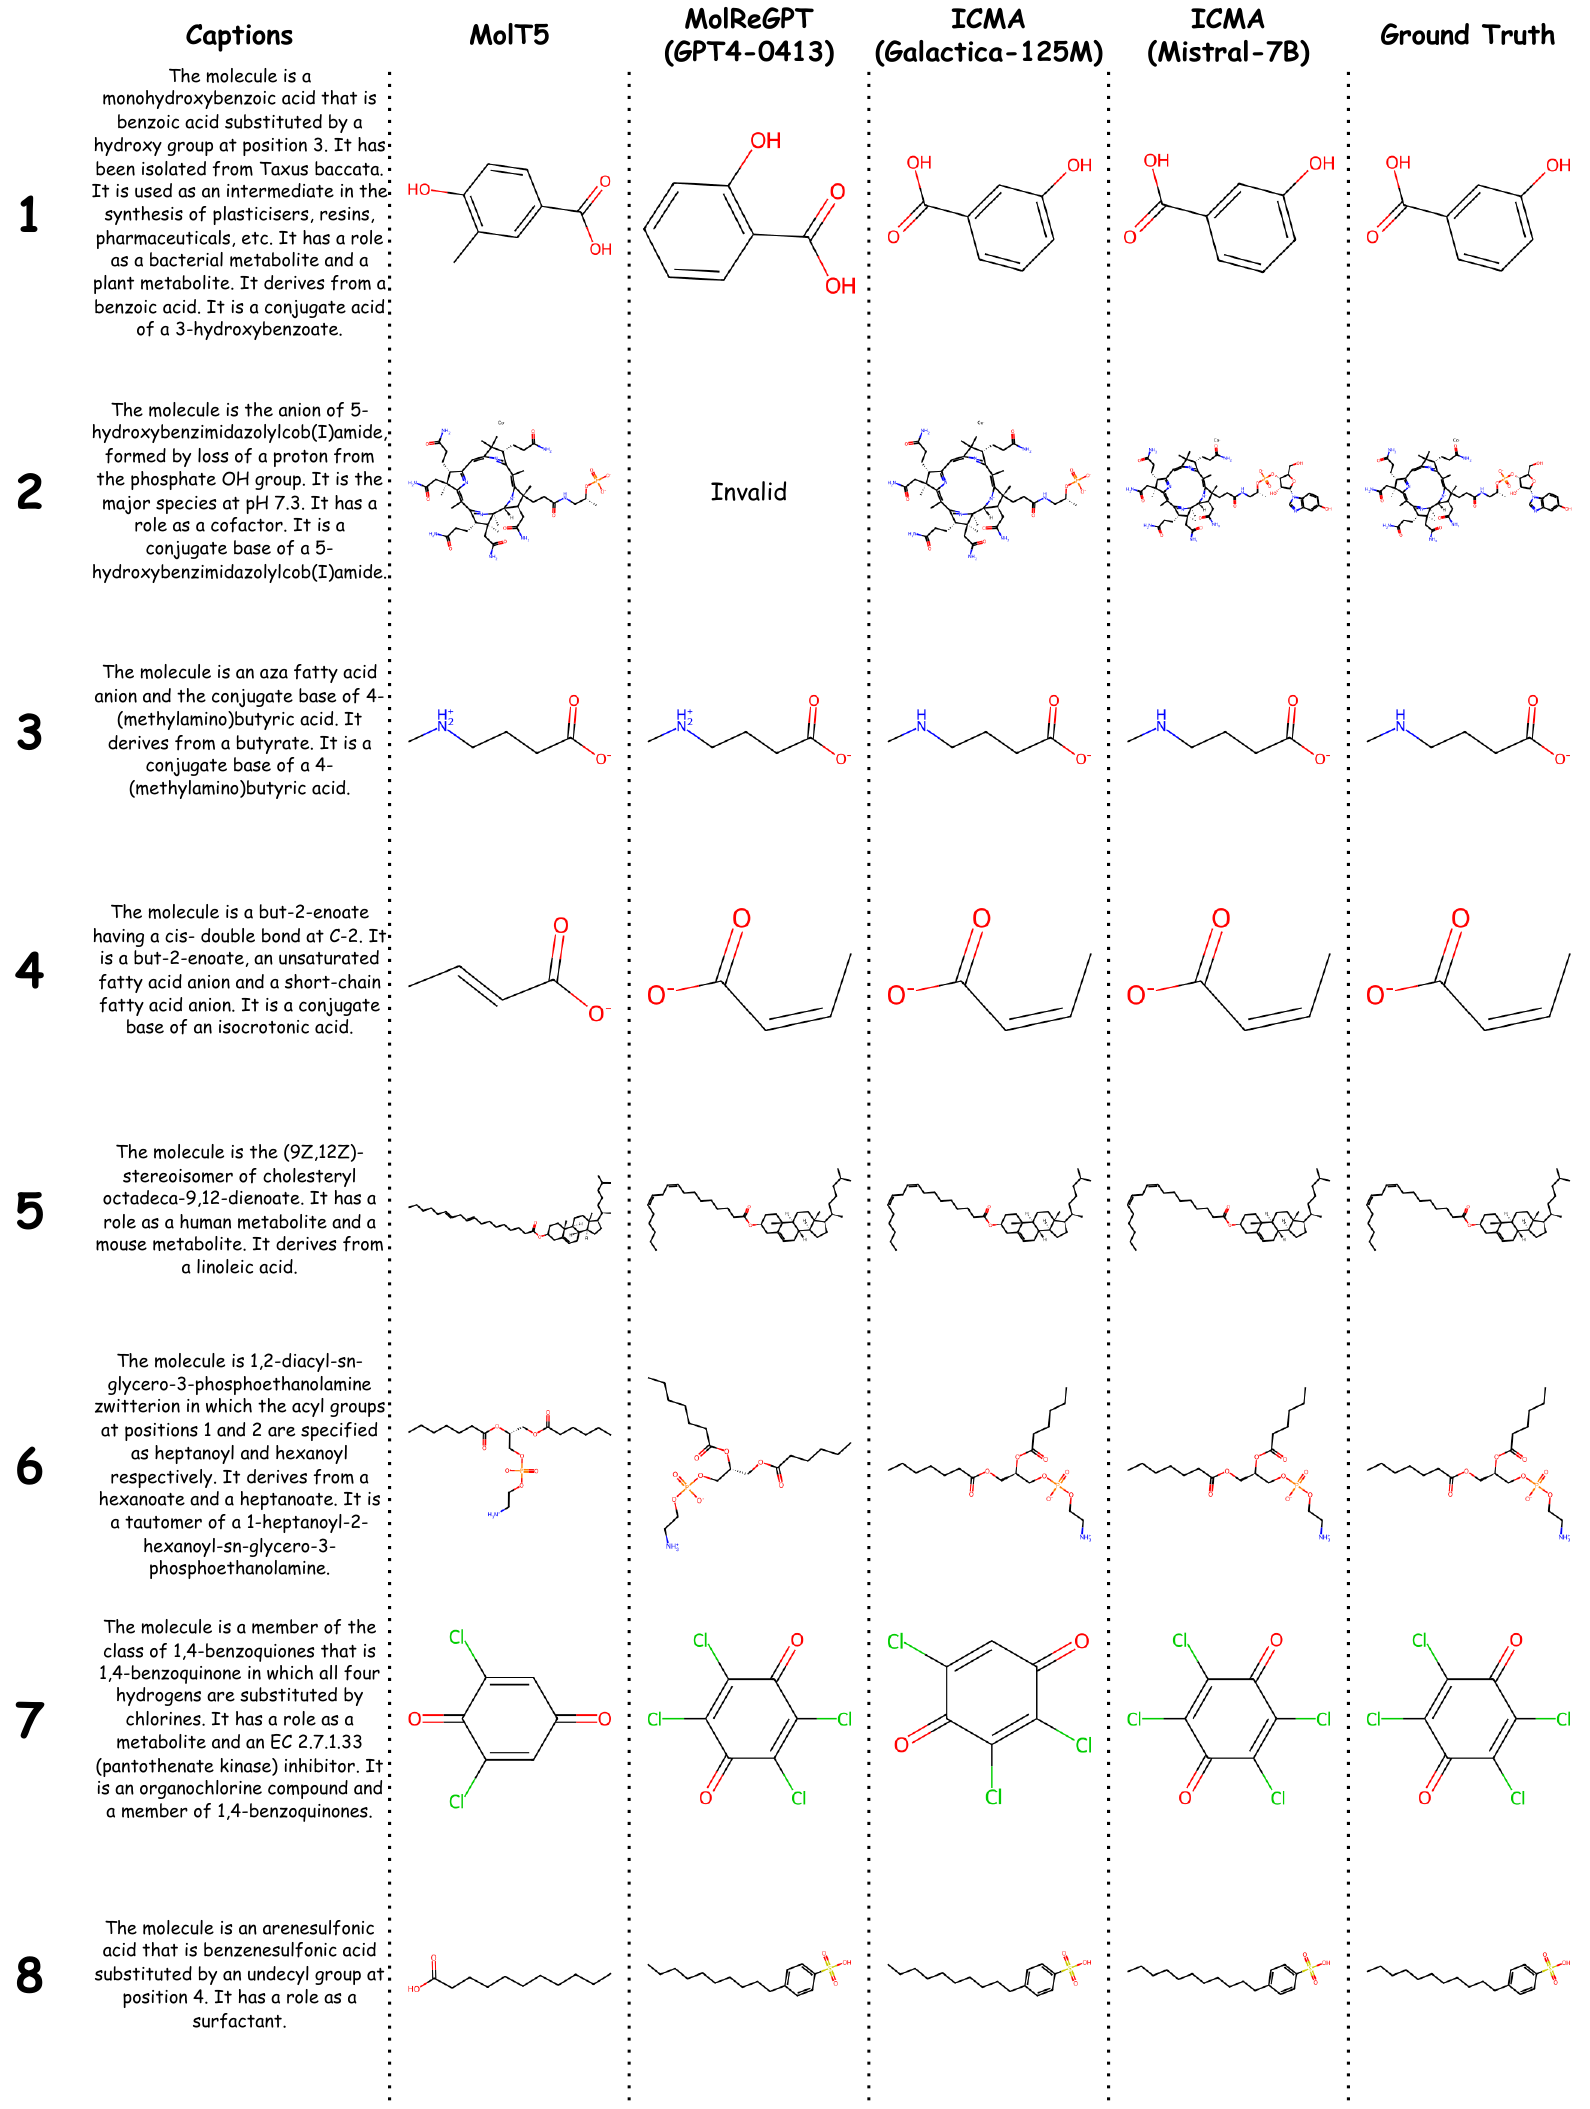}
    
    \caption{Molecule examples generated by different models based on the given captions in the Cap2Mol task.
    }
    \label{fig:case_c2m}
    
\end{figure*}

\begin{figure*}[htb]
    \centering
    
    \includegraphics[width=\textwidth]{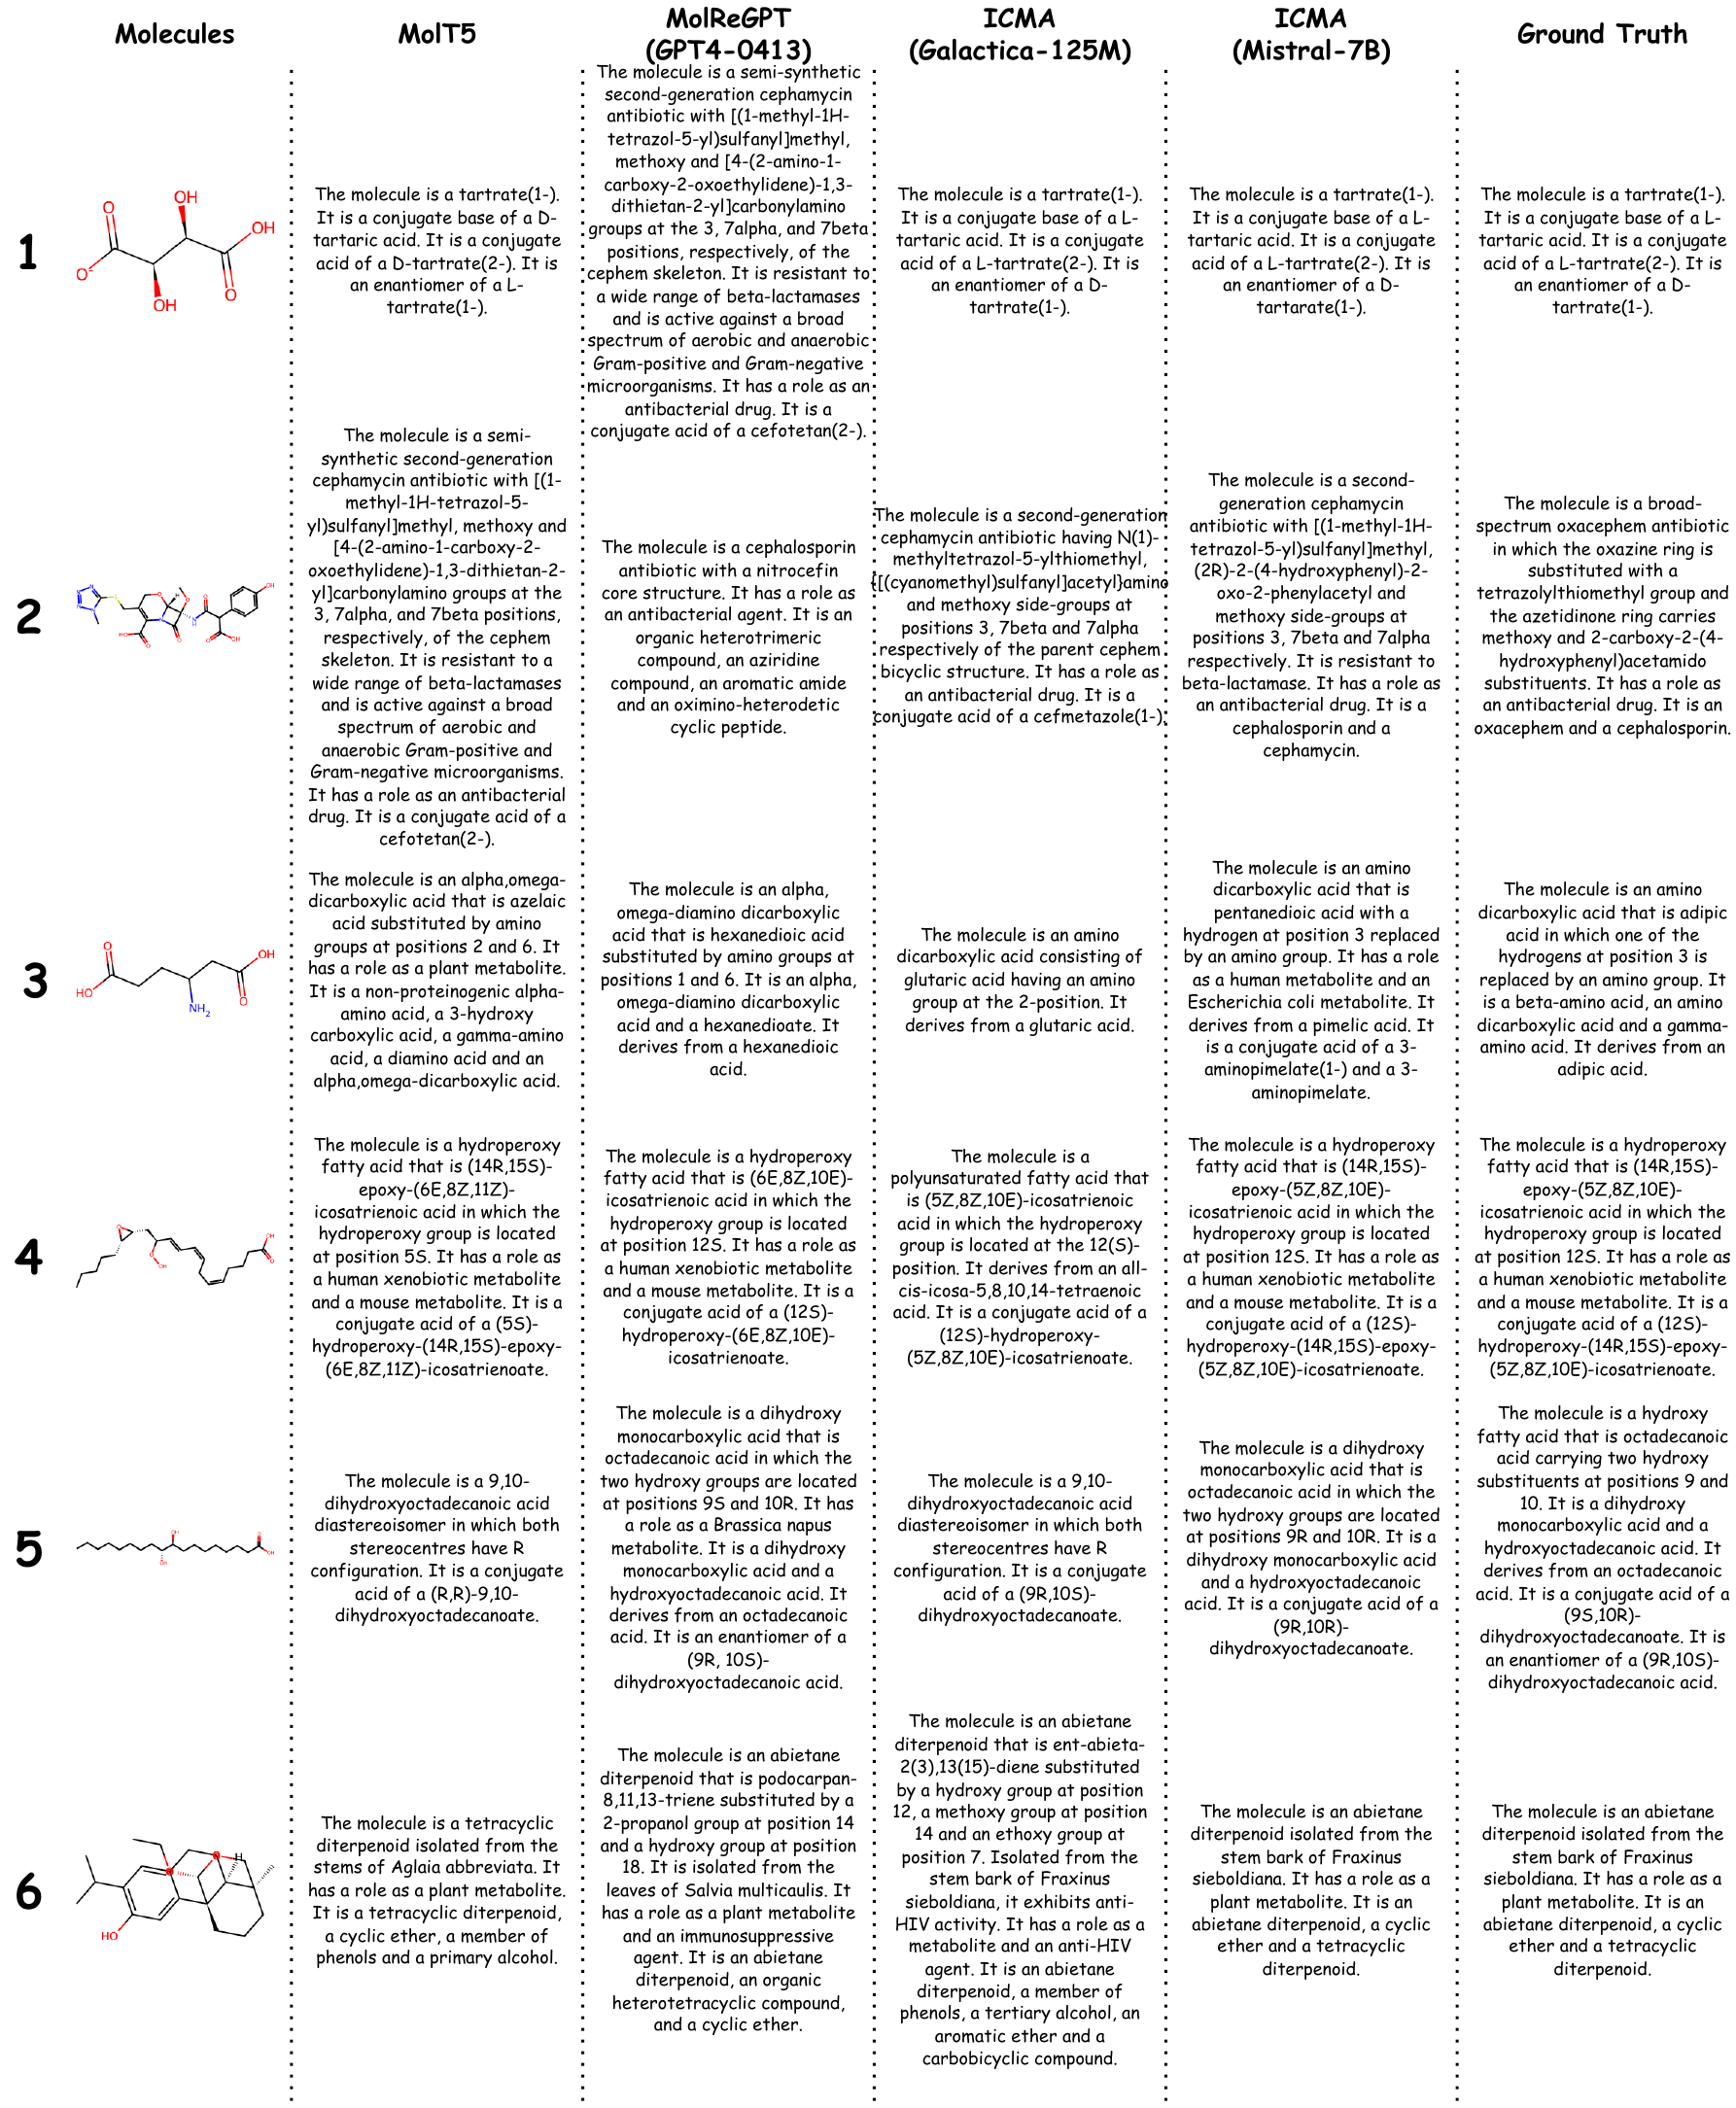}
    
    \caption{Caption examples generated by different models based on the given molecules in Mol2Cap task.
    }
    \label{fig:case_m2c}
    
\end{figure*}
